# Supplementary material for: Hybrid Functional Maps for Crease-Aware Non-Isometric Shape Matching
Source: arXiv:2312.03678 source file (2024-07-24)
Supplement: Supplementary file 1 [file suppl_non_orthogonality_analysis_fig.pdf]

Cougar 01

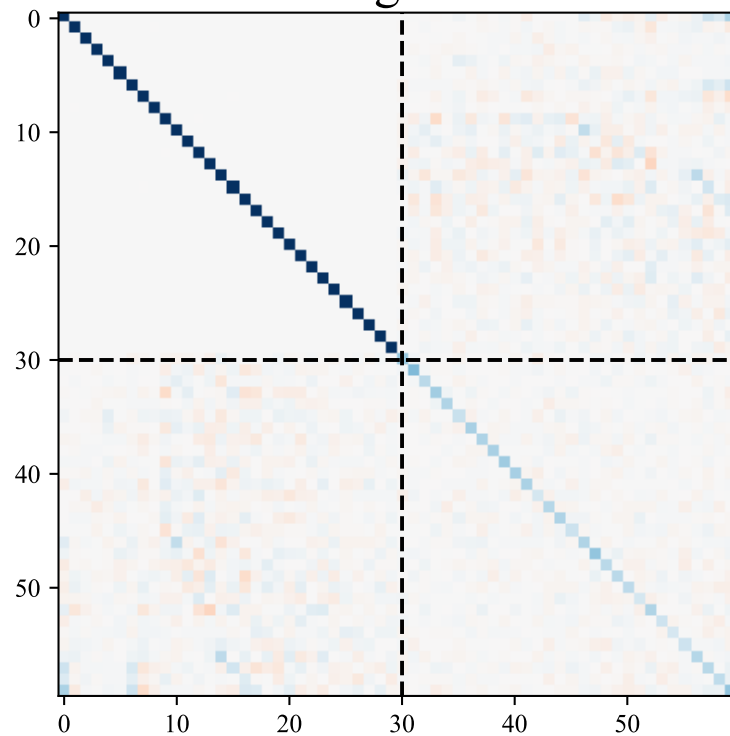

Horse 01

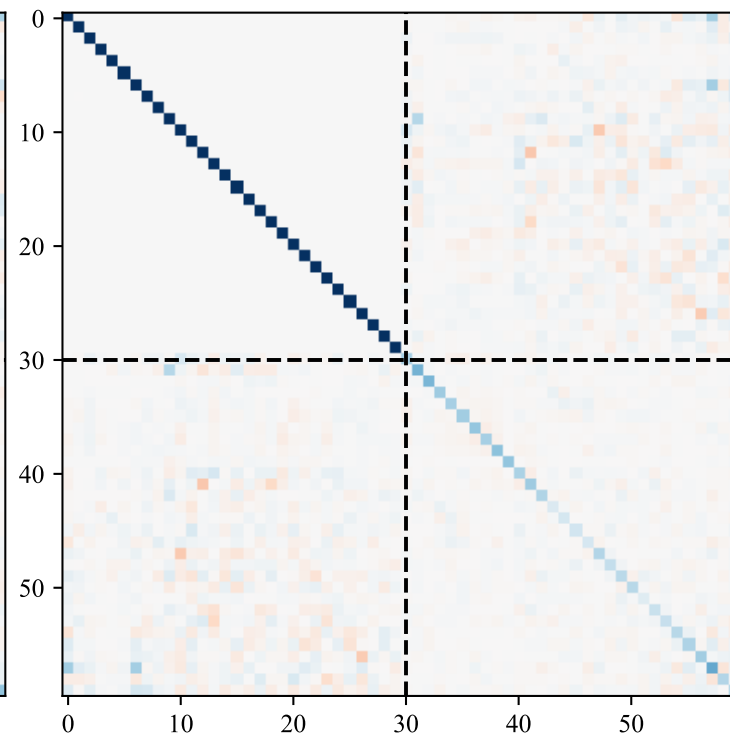

Hippo 01

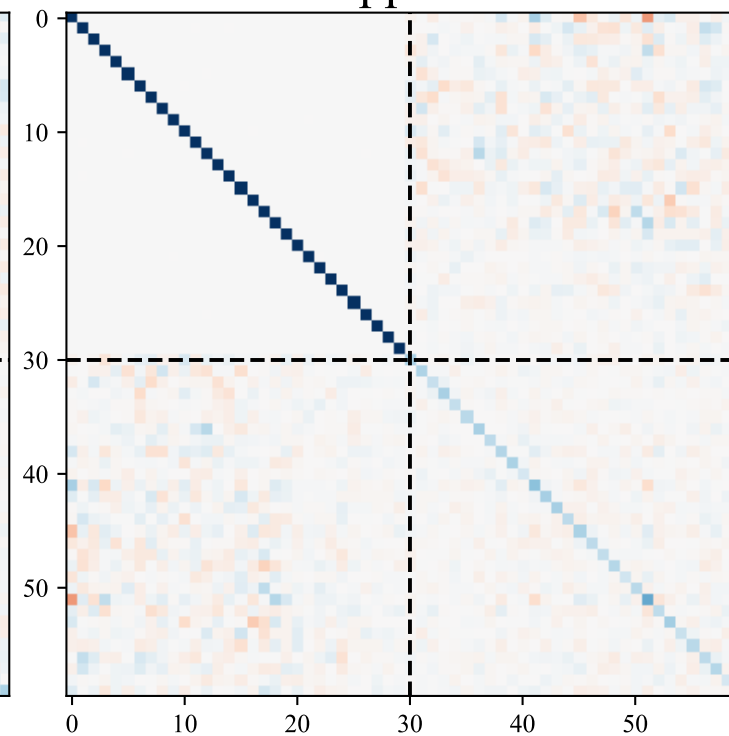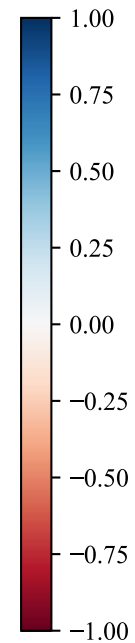 $\Phi$  $\Psi$

## Matrix of Inner Products
